# Supplementary material for: ReuseKNN: Neighborhood Reuse for Differentially-Private KNN-Based Recommendations
Source: arXiv:2206.11561 source file (2023-06-26)
Supplement: Supplementary file 1 [file generate_appendix.tex]

%%
%% This is file `sample-manuscript.tex',
%% generated with the docstrip utility.
%%
%% The original source files were:
%%
%% samples.dtx  (with options: `manuscript')
%% 
%% IMPORTANT NOTICE:
%% 
%% For the copyright see the source file.
%% 
%% Any modified versions of this file must be renamed
%% with new filenames distinct from sample-manuscript.tex.
%% 
%% For distribution of the original source see the terms
%% for copying and modification in the file samples.dtx.
%% 
%% This generated file may be distributed as long as the
%% original source files, as listed above, are part of the
%% same distribution. (The sources need not necessarily be
%% in the same archive or directory.)
%%
%% Commands for TeXCount
%TC:macro \cite [option:text,text]
%TC:macro \citep [option:text,text]
%TC:macro \citet [option:text,text]
%TC:envir table 0 1
%TC:envir table* 0 1
%TC:envir tabular [ignore] word
%TC:envir displaymath 0 word
%TC:envir math 0 word
%TC:envir comment 0 0
%%
%%
%% The first command in your LaTeX source must be the \documentclass command.
\documentclass[acmsmall]{acmart}
\usepackage{xcolor}
\usepackage{enumitem}
\usepackage{booktabs}
\usepackage{arydshln}
\usepackage{amsmath}
\usepackage{bbm}
\usepackage{bm}
\usepackage[ruled,vlined]{algorithm2e}
\usepackage{url}
\usepackage{float}
\usepackage[export]{adjustbox}
\usepackage{marvosym}
\usepackage{pifont}
\usepackage{multirow}
\usepackage{mathtools}
\usepackage{cancel}
\usepackage{stfloats}
\usepackage{multirow}
\usepackage{color, colortbl}
\usepackage{pdfpages}

\definecolor{Gray}{gray}{0.9}
\definecolor{DarkGreen}{rgb}{0.01, 0.75, 0.24}

%%
%% \BibTeX command to typeset BibTeX logo in the docs
\AtBeginDocument{%
  \providecommand\BibTeX{{%
    \normalfont B\kern-0.5em{\scshape i\kern-0.25em b}\kern-0.8em\TeX}}}

%% Rights management information.  This information is sent to you
%% when you complete the rights form.  These commands have SAMPLE
%% values in them; it is your responsibility as an author to replace
%% the commands and values with those provided to you when you
%% complete the rights form.
%\setcopyright{acmlicensed}
%\copyrightyear{2022}
%\acmYear{2022}
\acmDOI{XXXXXXX.XXXXXXX}
%\acmConference[ACM Transactions on Intelligent Systems and Technology]{ACM Transactions on Intelligent Systems and Technology}{2022}
%\acmBooktitle{ACM Transactions on Intelligent Systems and Technology}
\acmJournal{TIST}

%% These commands are for a PROCEEDINGS abstract or paper.
%\acmConference[Conference acronym 'XX]{Make sure to enter the correct conference title from your rights confirmation emai}{June 03--05, 2018}{Woodstock, NY}
%\acmPrice{15.00}
%\acmISBN{978-1-4503-XXXX-X/18/06}

%%
%% Submission ID.
%% Use this when submitting an article to a sponsored event. You'll
%% receive a unique submission ID from the organizers
%% of the event, and this ID should be used as the parameter to this command.
%%\acmSubmissionID{123-A56-BU3}

%%
%% For managing citations, it is recommended to use bibliography
%% files in BibTeX format.
%%
%% You can then either use BibTeX with the ACM-Reference-Format style,
%% or BibLaTeX with the acmnumeric or acmauthoryear sytles, that include
%% support for advanced citation of software artefact from the
%% biblatex-software package, also separately available on CTAN.
%%
%% Look at the sample-*-biblatex.tex files for templates showcasing
%% the biblatex styles.
%%

%%
%% The majority of ACM publications use numbered citations and
%% references.  The command \citestyle{authoryear} switches to the
%% "author year" style.
%%
%% If you are preparing content for an event
%% sponsored by ACM SIGGRAPH, you must use the "author year" style of
%% citations and references.
%% Uncommenting
%% the next command will enable that style.
%%\citestyle{acmauthoryear}

%\settopmatter{printacmref=true}

%%
%% end of the preamble, start of the body of the document source.
\begin{document}
    \includepdf[pages={26-29}]{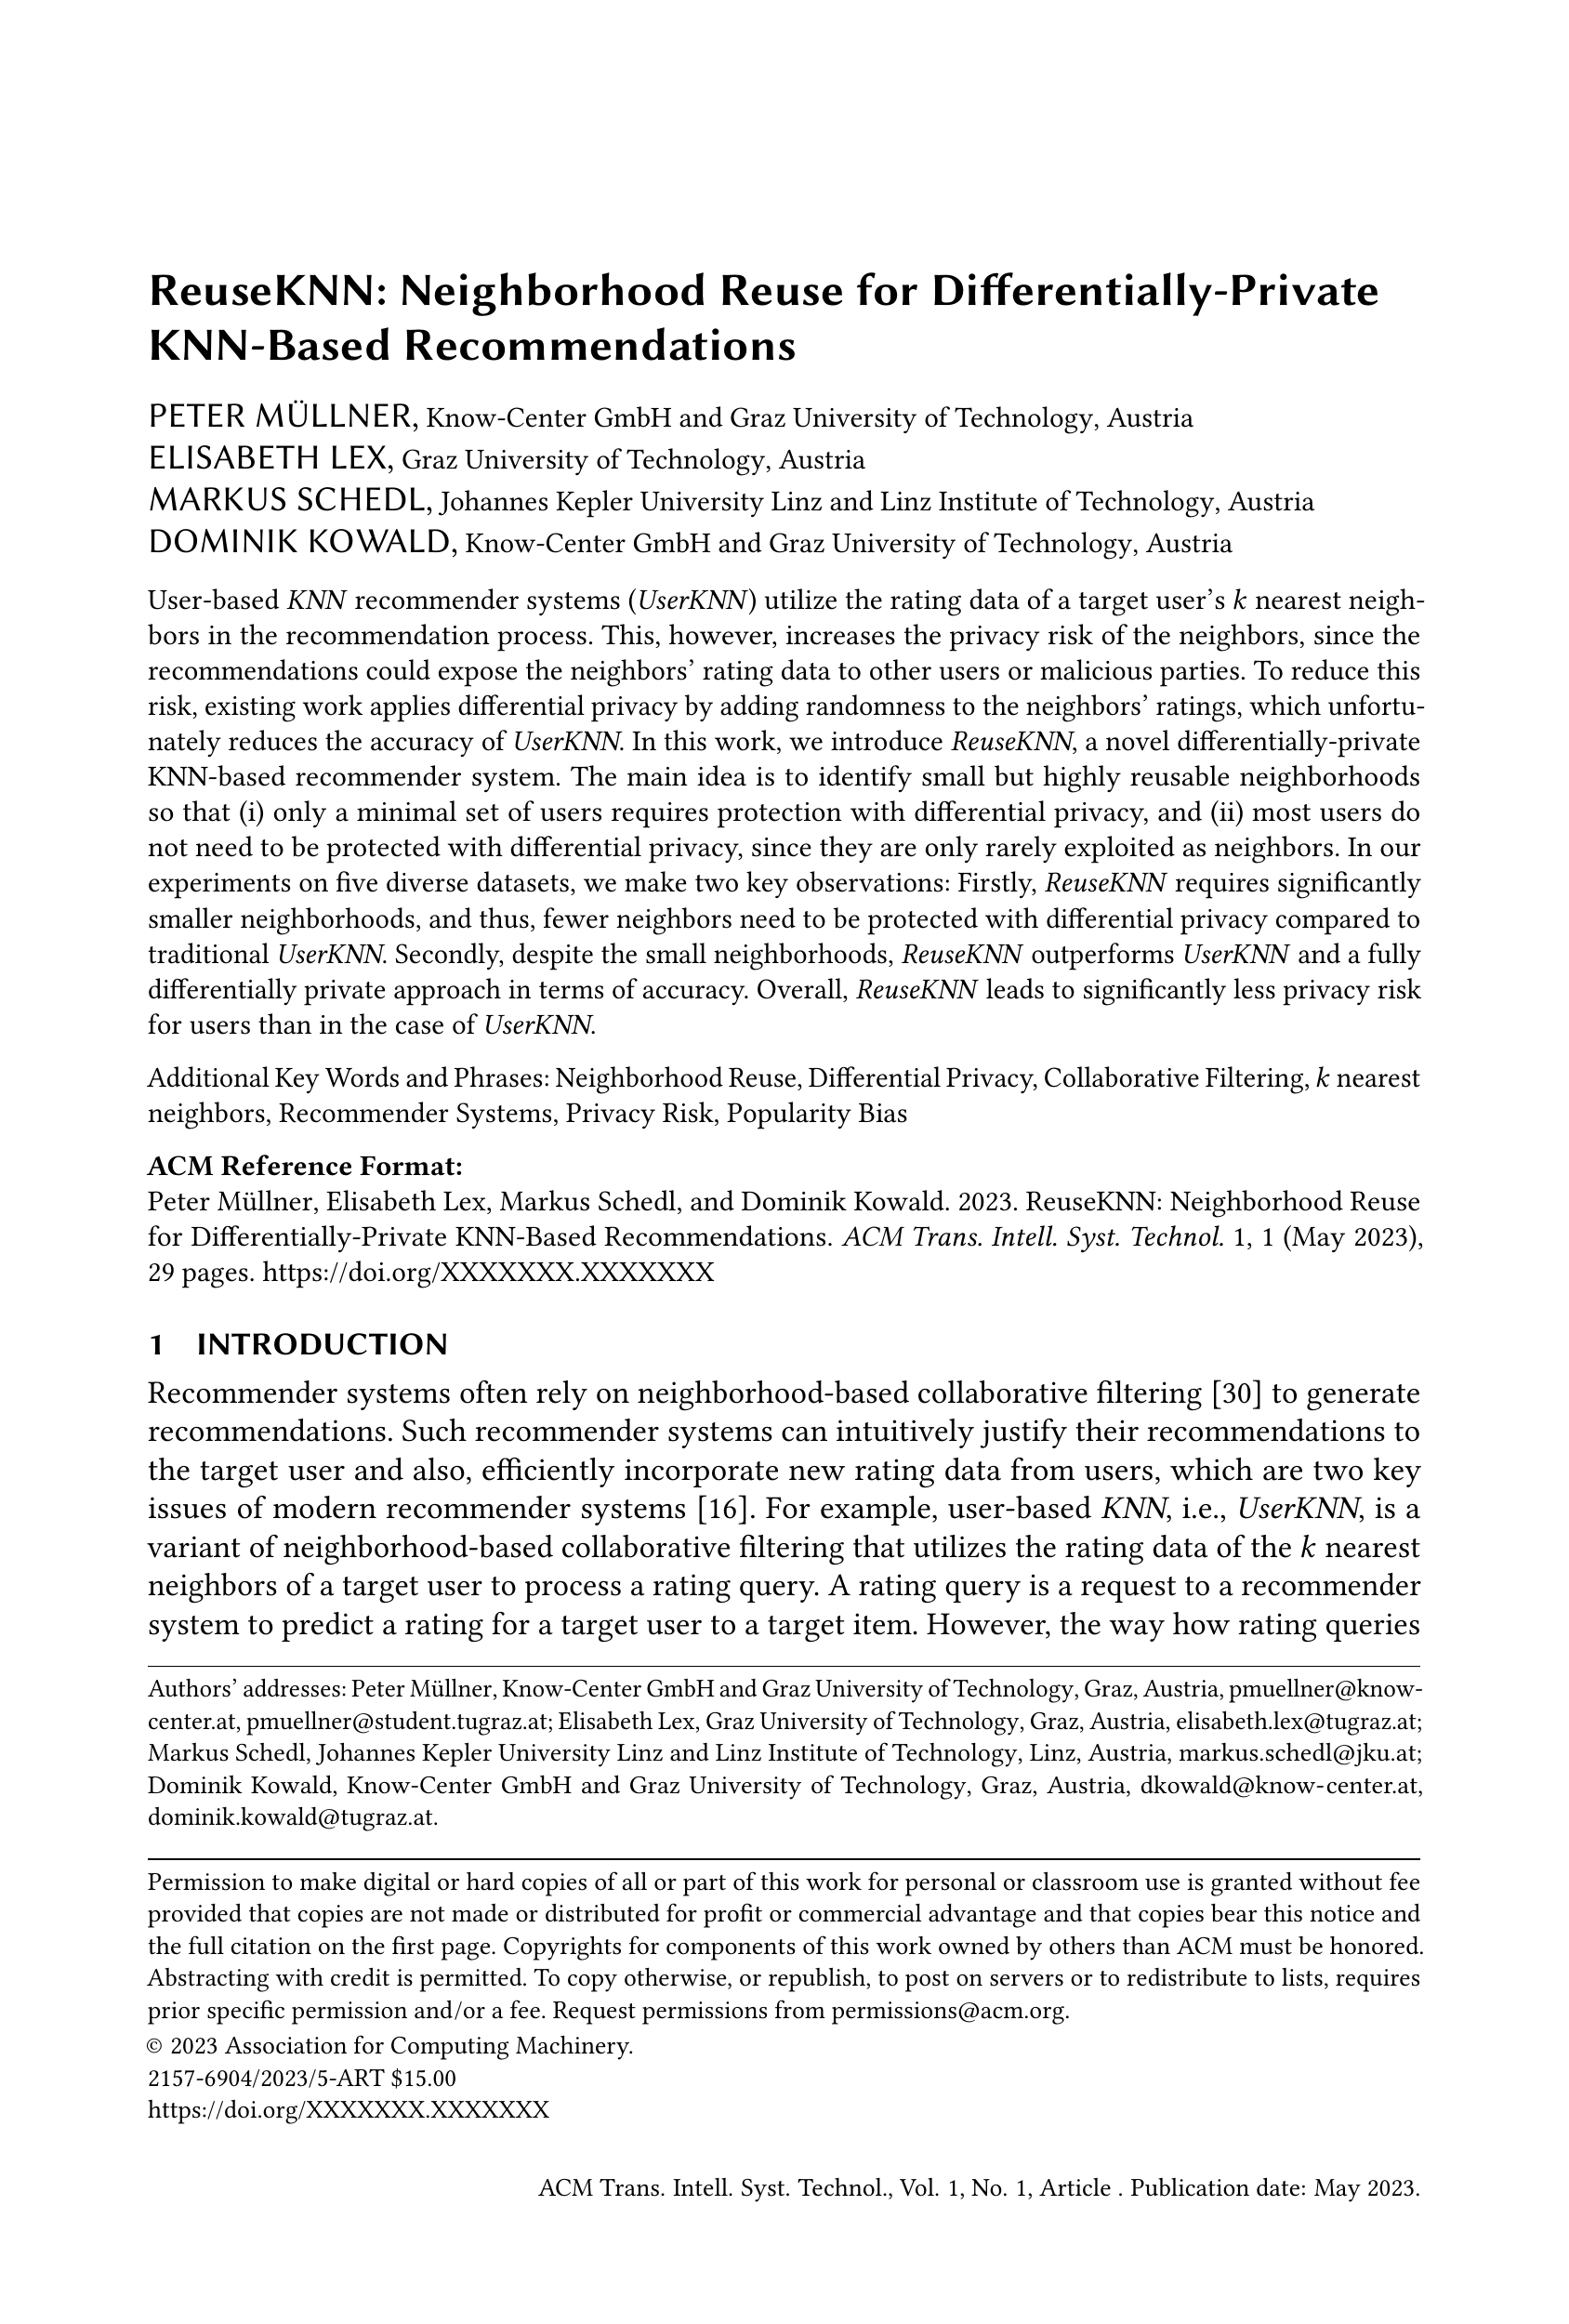}
\end{document}
